# Supplementary material for: A theoretical framework for the assessment of water fraction-dependent longitudinal decay rates and magnetisation transfer in membrane lipid phantoms
Source: arXiv:2408.17085 ancillary file (2024-08-30)
Supplement: Supplementary file 1 [file Supplementary_Information.pdf]

**Supporting information for:**  
**A theoretical framework for the assessment of water fraction-dependent longitudinal decay rates and magnetisation transfer in membrane lipid phantoms**

Heiko Neeb, Felix Schyboll, Rona Shaharabani, Aviv A. Mezer and Oshrat Shtangel

### **A. Three-pool Exchange Model**

The Bloch-equation for the three-pool model employed in the current work (Eqs. 1-3) contain a total of five free parameters. i.e. the equilibrium magnetisations of each pool ( $M_{0,L}$ ,  $M_{0,HW}$  and  $M_{0,FW}$ ) as well as the forward ( $k_{L,HW}$ ) and backward ( $k_{HW,L}$ ) exchange rates between lipid and hydration water. The  $R_1$  rates in Eqs. 1-3 were determined from the MD simulation ( $R_{1,L}$  and  $R_{1,HW}$ ) and from literature ( $R_{1,FW}$ ), whereas the exchange rate from hydration water to free water ( $k_{HW,FW}$ ) was set to a large fixed value such that the fast exchange condition between both water pools is met.

However, only three parameters are determined from a fit of the signal model to the experimental data: the magnetisation sum of all three pools,  $M_0$ , the hydration water concentration,  $f_{HW}$ , and the exchange rate between hydration water and lipid,  $k_{HW,L}$ . In the following, a detailed explanation for the relationship between the two parameter sets is given.

#### Equilibrium pool magnetisations

Starting point is the normalisation condition that the sum of all magnetisations in the Bloch-equation add up to one, i.e.

$$M_0 = M_{0,L} + M_{0,HW} + M_{0,FW} = 1. \quad (1')$$

It is important to note that the total water concentration,  $c_{H_2O}$ , has been determined independently in this work. As  $c_{H_2O}$  is given by the ratio of the signal measured in each voxel and the signal measured in voxels containing 100% water (after applying all relevant corrections for receiver inhomogeneity, saturation etc.), it is given by

$$c_{H_2O} = M_{0,HW} + M_{0,FW} \quad (2')$$

Thus, voxels containing only pure water ( $M_{0,L} = 0$ ) have a value of  $c_{H_2O} = 1$ , as expected, whereas  $M_{0,L} = 1$  for voxels with  $c_{H_2O} = 0$ .

Using Eqs. 1' and 2', the magnetisation of the MR invisible lipid pool is thus given by

$$M_{0,L} = M_0(1 - c_{H_2O}). \quad (3')$$

Now, employing Eq. 3' and the definition of the hydration water fraction,  $f_{HW} = M_{0,HW}/M_{0,L}$ , the equilibrium magnetisation of the hydration water pool becomes

$$M_{0,HW} = f_{HW} M_{0,L} = f_{HW} M_0 (1 - c_{H_2O}). \quad (4')$$

Plugging Eq. 4' into Eq. 2' finally results in the equilibrium magnetisation of the free water pool,

$$M_{0,FW} = M_0 (c_{H_2O} - f_{HW} (1 - c_{H_2O})) \quad (5')$$

### Exchange rates

The principle of detailed balance provides a relationship between the forward and the backward magnetisation exchange rates between lipid and hydration water,

$$M_{0,L} k_{L,HW} = M_{0,HW} k_{HW,L} \quad (6')$$

Once again employing  $f_{HW} = M_{0,HW} / M_{0,L}$ , the latter equation can be written as,

$$k_{L,HW} = k_{HW,L} f_{HW} \quad (7')$$

Finally, the principle of detailed balance also determines the exchange rate between free water and hydration water, given the assumed known and fixed value for  $k_{HW,FW}$ ,

$$M_{0,FW} k_{FW,HW} = M_{0,HW} k_{HW,FW} \quad (8'),$$

which transforms to (using Eq. 4' and 5'),

$$k_{FW,HW} = \frac{f_{HW}(1 - c_{H_2O})}{c_{H_2O} - f_{HW}(1 - c_{H_2O})} k_{HW,FW} \quad (9')$$

## **B. Normalisation of MR data**

To fit the model (Eqs. 1-3) to the experimental SPGR datasets, the latter have to be properly normalised in order to comply with the normalisation conditions imposed by the signal model, i.e. Eqs. 1' and 2'. This was ensured by the following preprocessing steps (all steps were performed individually for each of the four SPGR measurements):

1. Apply receiver correction
2. Determine the average signal intensity in voxels with  $c_{H_2O} = 1$ . Let call this quantity  $\overline{M_0}(c_{H_2O} = 1)$ .
3. Normalise each dataset by dividing by  $\overline{M_0}(c_{H_2O} = 1)$ .

This results in a normalisation of the SPGR datasets such that Eqs. 1' and 2' are fulfilled.

### C. Proton density distributions in lipids and the associated water pools

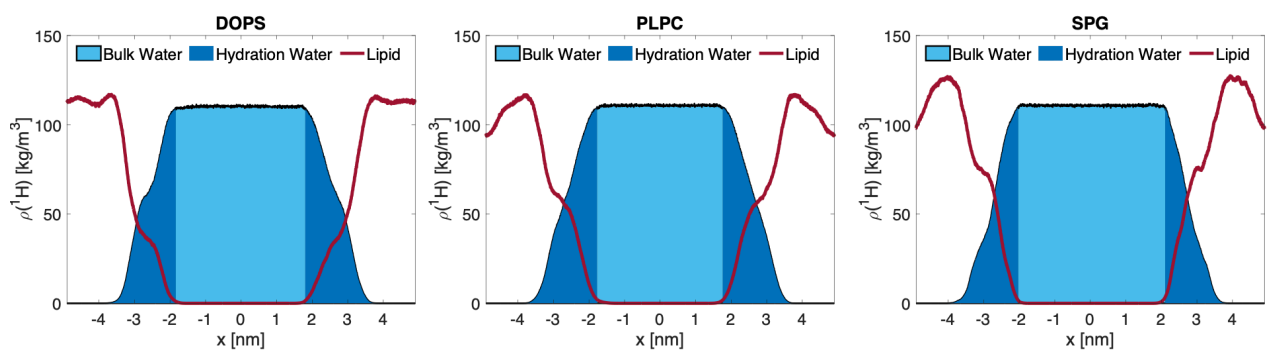

Figure S1: Proton density distribution along the bilayer normal (x-axis) for DOPS, PLPC and SPG (red lines). The corresponding proton density of the water pool is shown as a filled blue area. The latter is divided into hydration water (dark blue) and free water (light blue) as described in the text.

### D. Workflow for the validation of the three-pool model fit

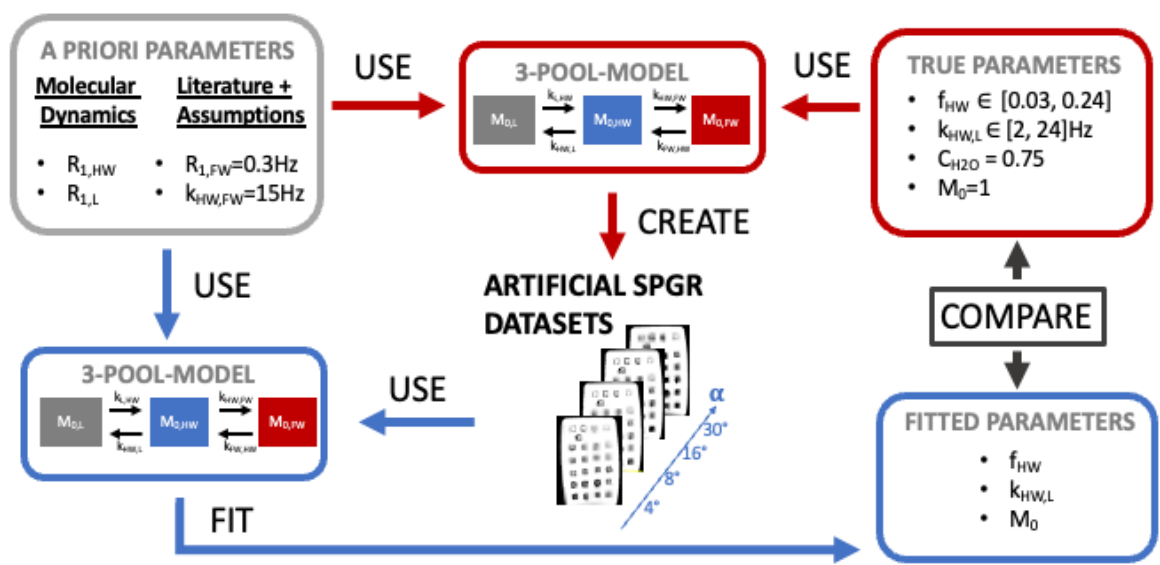

Figure S2: Workflow employed for the validation of the three-pool model. Pool-specific relaxation rates were determined as described in the main text. Based on these parameters, artificial noisy SPGR datasets at four different flip angles were created for different values of  $f_{HW}$  and  $k_{HW,L}$ , which were subsequently employed to fit  $f_{HW}$ ,  $k_{HW,L}$  and  $M_0$ , in complete analogy to the processing of real data. The fitted values were then compared to the corresponding true values.

### E. Results from a fit to the data without the $\alpha = 30^\circ$ measurement

Table S1 and Figures S3 and S4 contain the results obtained for the reduced dataset where only three flip angles were included,  $\alpha \in [4^\circ, 8^\circ, 16^\circ]$ . The results shown here have to be compared to the corresponding results obtained with the full dataset, including the  $\alpha = 30^\circ$  measurement and shown in Tab. 1 and Figs. 2 and 3 of the main manuscript.

|         | Model Fit to Experimental Data |                       |                                    |                                 |
|---------|--------------------------------|-----------------------|------------------------------------|---------------------------------|
|         | $N_{\text{Curv}}$              | $\bar{f}_{\text{HW}}$ | $\bar{k}_{\text{L,HW}}[\text{Hz}]$ | $\bar{k}_{\text{t}}[\text{Hz}]$ |
| PLPC    | 33 (39)                        | 0,088<br>$\pm 0,006$  | 1,7<br>$\pm 0,4$                   | 0,019<br>$\pm 0,04$             |
| DOPS    | 12 (14)                        | 0,15<br>$\pm 0,02$    | 8,3<br>$\pm 2,8$                   | 0,23<br>$\pm 0,05$              |
| SPG     | 13 (13)                        | 0,19<br>$\pm 0,01$    | 2,8<br>$\pm 0,6$                   | 0,12<br>$\pm 0,03$              |
| PC-Chol | 30 (35)                        | 0,16<br>$\pm 0,01$    | 5,1<br>$\pm 0,8$                   | 0,12<br>$\pm 0,02$              |
| PS-SPG  | 6 (7)                          | 0,16<br>$\pm 0,02$    | 10,4<br>$\pm 4,2$                  | 0,19<br>$\pm 0,04$              |

**Table S1:** Results from the three-pool model fit to the spoiled gradient echo data for the different lipids and lipid mixtures. Here, in contrast to Tab. (1) in the main manuscript, the  $\alpha = 30^\circ$  has been omitted from the fit. The results were based on the numbers of cuvettes that could be fitted ( $N_{\text{Curv}}$ ), whereas the total number of measured cuvettes is given in brackets.  $\bar{f}_{\text{HW}}$  is the average hydration water fraction obtained by the fit of the three-pool model,  $\bar{k}_{\text{HW,L}}$  characterizes the average exchange rate between hydration water and lipid (relative to the hydration water pool size) and  $\bar{k}_{\text{t}}$  is the corresponding exchange rate normalized to the total magnetisation of all pools.

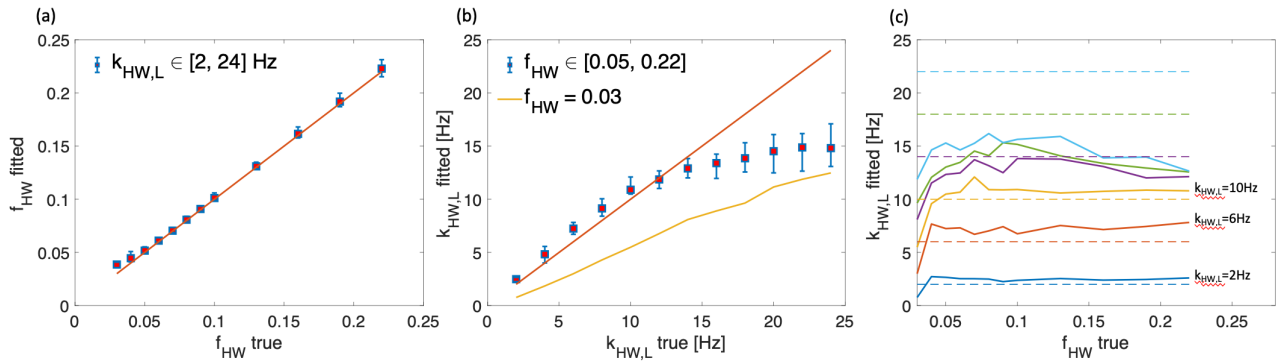

**Figure S3:** Results from the validation of the three-pool model. Here, in contrast to Fig. (2) in the main manuscript, the  $\alpha = 30^\circ$  has been omitted from the fit. (a) shows the fitted hydration water fraction versus the true value of  $f_{\text{HW}}$  for different exchange rates,  $k_{\text{HW,L}}$ . The corresponding results for the exchange rate

between hydration water and lipid is shown in (b). Data were averaged over hydration water fractions ranging in the interval  $[0.05 \text{ } 0.22]$ . In addition, the orange line shows the results for a small  $f_{\text{HW}} = 0.03$ , which clearly deviates from the results at  $f_{\text{HW}} \geq 0.05$ . In both (a) and (b), the red line shows the identity of fitted and true parameter values. To further illustrate the interdependence between  $f_{\text{HW}}$  and  $k_{\text{HW,L}}$ , (c) shows the fitted results of the exchange rate as a function of hydration water fraction for different true values of  $k_{\text{HW,L}}$  (colored lines).

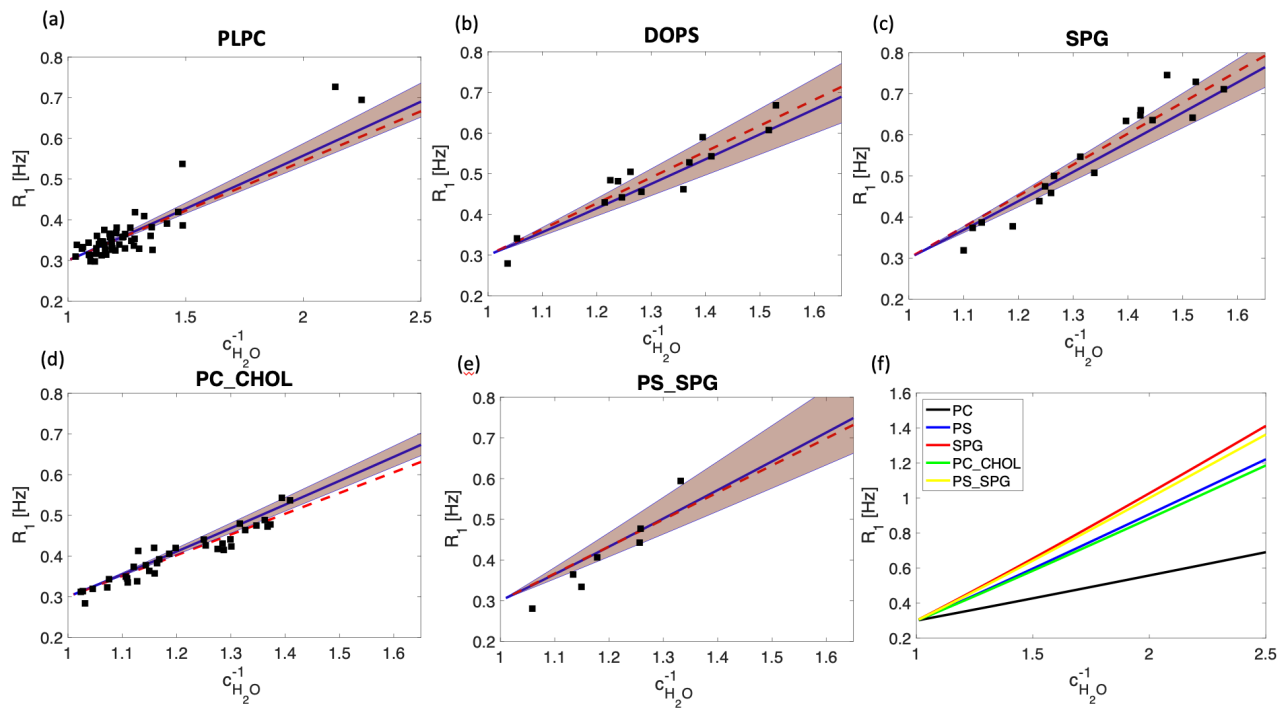

**Figure S4:**  $R_1$ -relaxivity of different lipids and lipid mixtures. Here, in contrast to Fig. (3) in the main manuscript, the  $\alpha = 30^\circ$  has been omitted from the fit. The dependence of  $R_1$  on the inverse water concentration is shown for (a) PLPC, (b) DOPS, (c) SPG, (d) PC-Chol and (e) PS-SPG. The filled boxes show the experimental results of individual cuvettes, while the blue curves present the prediction of the three-pool exchange model. The uncertainty of the predicted  $R_1$  is covered by the filled red area. Note that the uncertainty increases with decreasing water concentration for all lipids and lipid mixtures investigated. Moreover, the results from a straight line fit to the data are superimposed as dashed red lines. The slopes of those lines define the hydration water fraction in the FPD model (see text). For a better and direct comparison, the three-pool model predictions for all lipids and mixtures are shown in (f).
